# Supplementary material for: Anomaly Detection in Big Data
Source: arXiv:2203.01684 source file (2022-03-03)
Supplement: Supplementary file 1 [file Appendix.tex]

\thispagestyle{empty}
\chapter{Supplementary Material}
\section{Convex Sets and Functions}
A set $\mathcal{C} \in \mathcal{R}^n $ is convex if for any two elements ${\bf x, y} \in \mathcal{C}$, we have $\theta {\bf x} + (1-\theta){\bf y} \in \mathcal{C}$ where $\theta \in [0,1]$. Intuitively, line segment joining ${\bf x}$ and ${\bf y}$ lies completely within the set $\mathcal{C}$. Some examples of convex sets are line,  disk, half-space, hyperplane etc. A function $f$ is said to be convex over a convex set $\mathcal{C}$ if the line segment joining any two points $({\bf x}, f({\bf x}))$ and $({\bf y}, f({\bf y}))$ lies completely above the graph of the function. Formally,
\begin{equation}
f(\theta {\bf x} + (1-\theta){\bf y}) \leq \theta f({\bf x}) + (1-\theta)f({\bf y}) \;\;\; \theta \in [0,1]. 
\end{equation}
Some examples of convex functions are norm ball $\{{\bf x} \in \mathcal{R}^n| \|{\bf x}\|_p \leq t, t \in \mathcal{R} \}$ for any norm $p \geq 1$, square function $x^2$, absolute value function $|x|$ etc. 

The most fundamental property of convex functions is stated in the following theorem without proof (for proof,  please ref. to  \cite{Boyd:2004}):
\begin{thm}
For a convex function,  a local minima is a \emph{global} minima.
\end{thm}
\section{Lipschitz Function and Strong Convexity}\label{smoothstrong}
A function $f$ is said be lipschitz continuous if the gradient of $f$ at a point ${\bf x} \in \mathcal{R}^n$ is bounded. Intuitively, this means that small change in input does not cause huge change in output.  More formally, 
\begin{equation}
\|f({\bf x}) -f({\bf y})\|  \leq L \|{\bf x} -{\bf y}\|  
\end{equation}
where $L >0$ is called lipschitz constant and norm  used is general norm; ${\bf x},{\bf y} \in \mathcal{R}^n$. 

A function $f$ is said to be strongly convex with parameter $\mu$ iff the function  ${\bf x} \mapsto f({\bf x}) -\frac{\mu}{2}\|{\bf x}\|^2 $ is convex.
Intuitively, strongly convex gives an indication about the curvature of the function. Large positive $\mu$ means the function has positive curvature and so on.
\section{Norm and Dual Norm}\label{norm}
A norm is a function $\|\cdot\|$ from the a vector space to the real numbers  that satisfies the following properties:
\begin{itemize}
\item {\bf Non-negativity:} For any $\|{\bf x}\| \geq 0$.
\item {\bf Absolute Homogeneity} For any scalar $t$, $\|t{\bf x}\| = |t|\|x\|$. 
\item {\bf Triangle Inequality} For any two vectors ${\bf x}$, ${\bf y}, \|{\bf x}+{\bf y}\| \leq \|{\bf x}\| + \|{\bf y}\|$.
\end{itemize}

Dual norm is analogously defined. 
\begin{equation}
\|{\bf y}\|_* = \text{sup} \{{\bf x}^T{\bf y} | \|{\bf x}\| \leq 1\}
\end{equation}
Intuitively, it measures the size of ${\bf y}$ with respect to the size (norm) of ${\bf x}$.

\section{Positive-Definiteness}\label{psd}
A matrix $X$ is said to be semi-positive definite if for any nonzero vector ${\bf z}$, the following condition is satisfied:
\begin{equation*}
\centering 
{\bf z}^TX{\bf z} \geq 0
\end{equation*}
The matrix $X$ is said to be positive-definite if the above inequality is \emph{strict}. In other words, a semi-definite (definite) matrix $X$ has all its eigen value $\geq 0$ (>0). 

\section{Mercer's Condition}\label{mercer}
A real-valued function $\kappa ({\bf x},{\bf z})$ satisfies Mercer's condition if  $\forall$ square integrable functions $h({\bf x},{\bf z}) $
\begin{equation*}
\int \int h({\bf x})\kappa({\bf x},{\bf z})h({\bf z})d{\bf x}d{\bf z} \geq 0
\end{equation*}
 Mercer's condition ensures that the kernel function $\kappa({\bf x},{\bf z})$ is a valid positive-definite function.

\section{Johnson-Lindenstrauss Lemma}\label{jl}
Informally, Johnson-Lindenstrauss Lemma states that a collection of points in a high dimension space can be embedded to a much lower dimension subspace such that the distances between points are \emph{nearly preserved}.

Formally,Given $0<\epsilon<1$, a set \emph{S} of $n$ points in $\mathcal	{R}^N$, and a number $m>8\frac{ln(n)}{\epsilon}^2$, there exists a linear function $g:\mathcal{R}^N \mapsto \mathcal{R}^n$ such that 
\begin{equation}
(1-\epsilon)\|x-y\|^2  \leq \|g(x)-g(y)\|^2 \leq (1+\epsilon)\|x-y\|^2
\end{equation}
for all $x,y \in \emph{S}$.
